# Supplementary material for: Energy-efficient operation of neural operators for virtual sensing
Source: arXiv:2609.30580 source file (2026-09-24)
Supplement: Supplementary file 1 [file inventory.tex]

\documentclass{article}

\IfFileExists{PRIMEarxiv.sty}
  {\def\OpCertProjectRoot{}}
  {\def\OpCertProjectRoot{../}}
\makeatletter
\edef\input@path{{\OpCertProjectRoot}}
\makeatother
\usepackage[utf8]{inputenc}
\usepackage[T1]{fontenc}
\usepackage{PRIMEarxiv}
\usepackage{enumitem}
\usepackage[dvipsnames]{xcolor}
\usepackage{hyperref}
\hypersetup{colorlinks=true,linkcolor=Blue,urlcolor=Blue}
\pagestyle{empty}
\begin{document}
\begin{center}
{\large\bfseries Inventory of Supporting Information}\\[2pt]
{\small Energy-efficient virtual sensing of physical fields with edge-deployed neural operators}
\end{center}
\vspace{8pt}

\noindent\textbf{Main and Extended Data figures.} Four main figures report reuse, complete-service energy, operator structure and operating costs. Three Extended Data figures resolve service-phase energy, the reuse mechanism and worker replacement.

\noindent\textbf{Supplementary Information.} Eleven notes, 21 tables and five figures support the main results. The opening guide links each main-text comparison to its supporting note.
\begin{enumerate}[leftmargin=2em,itemsep=2pt,label=\textbf{Supplementary Note \arabic*.}]
  \item Heat-exchanger execution costs and source comparison.
  \item Heat-exchanger service energy and execution controls.
  \item Response latency and request energy.
  \item Computation and service-path profiling.
  \item Physical decoding and prediction error.
  \item Operator coverage and prepared-input reuse costs.
  \item Numerical references and comparison scope.
  \item Qualification and execution controls.
  \item Resource history and worker recovery.
  \item Alternative numerical criteria and recovery controls.
  \item Field reconstruction, missed updates and recovery.
\end{enumerate}

\noindent\textbf{Supporting materials.} Figure data, original execution records, profiling traces and reproduction code are available to editors and reviewers from the corresponding author on request during peer review, as stated in Data and Code availability.
\end{document}
